# Supplementary material for: Is Image Memorability Prediction Solved?
Source: arXiv:1901.11420 source file (2019-01-31)
Supplement: Supplementary file 1 [file appendix.tex]

\section{Appendix:   The Validity of Memorability Scores}
\label{apdx:variance}

The upper bound on LaMem is the mean rank correlation between the memorability scores corresponding to different groups of people. 
As our solution reached this upper bound, we ask ourselves whether the memorability scores, obtained through the Memory Game described in Section~\ref{sec:related-work}, form a sufficient representation. 
We explore two key questions. The first is whether the variance across observers should also be considered. The second is whether the order in which the images are displayed is important.

\vspace{-0.2in}
\subsubsection{Are the scores a good representation?}

%1. Describe the practice
The existing datasets assumed that it suffices to characterize an image by a single score, which indicates how often participants correctly detect a repetition of the image.
Is this the right practice? 
How do the memorability scores vary across groups of observers?
%To convince ourselves that the memorability scores we rely on are valid we 
To answer these questions, we examined the role of the variance across groups of people.

%2. What we did to challenge the above
Specifically, we measured the variance of the memorability scores given by different groups of people, per image.
We measured the variance across groups of the same size, for varying group sizes---from $40$ to $130$.
% The scores were computed for groups of varying sizes --- from $40$ to $130$.
This was done for 45 images.
%, described in Section~\ref{subsec:observers}.

%3. Our experiment results
Figure~\ref{fig:variance} shows our results.
Every point in the graph represents a different image.
A couple of conclusions can be drawn from this graph.
First, the variance depends on the memorability. 
The more memorable an image, the smaller the variance.
It means that people tend to agree on what makes an image memorable, proving that it suffices to maintain only one number---the memorability score---which is the common practice.

A second conclusion from Figure~\ref{fig:variance}, is that the larger the number of participants, the smaller the variance across groups. 
This could be useful for future work, suggesting that a larger number of observers per image could lead to more stable scores, with higher human consistency.

%This supports our observation from Section~\ref{subsec:observers}.

% %4. What we suggest
% While the second observation was expected, the first one was rather surprising.
% When we started the study, we believed that the variance will tell us a different story than the memorability score, and both would have to be maintained.
% However, Figure~\ref{fig:variance} proves that it suffices to maintain only one number---the memorability score---which is what is the common practice.

\begin{figure}[!ht]
\includegraphics[width=0.37\textwidth]{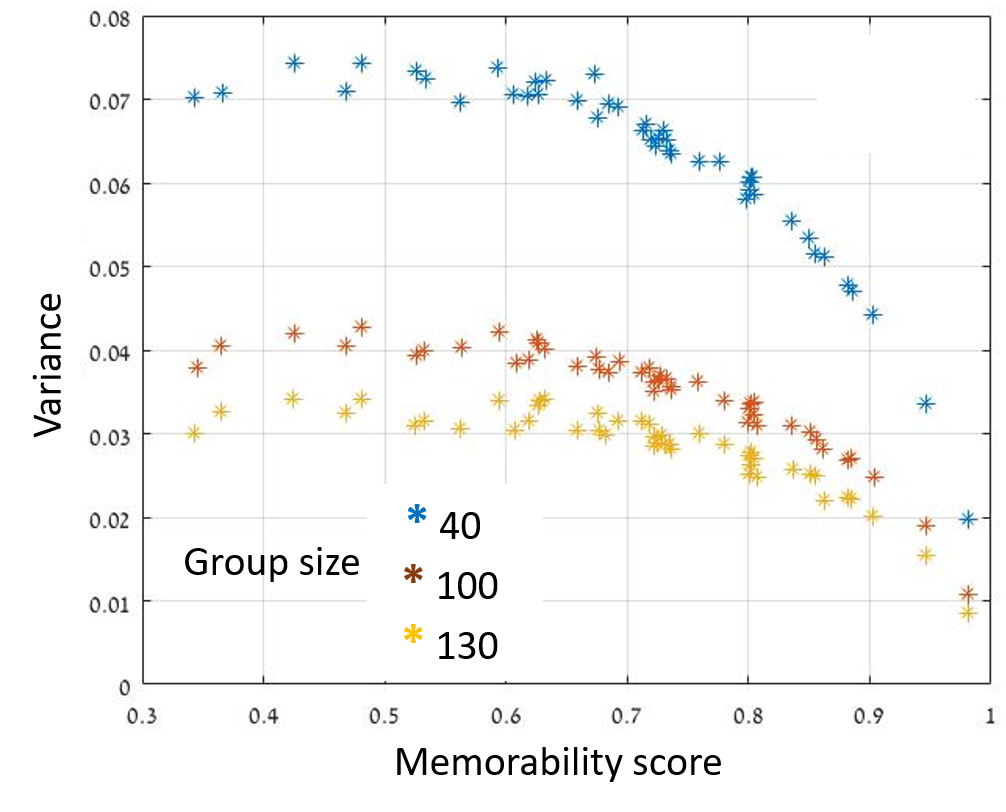}
\centering\caption{{\bf Memorability variance depends on the memorability score.} Variance decreases as memorability score increases. Variance also decreases for a larger participants' group size.}
\label{fig:variance}
\end{figure}

\begin{figure*}[!htb]
\centering
  \begin{subfigure}[b]{\textwidth}
  \includegraphics[width=\textwidth]{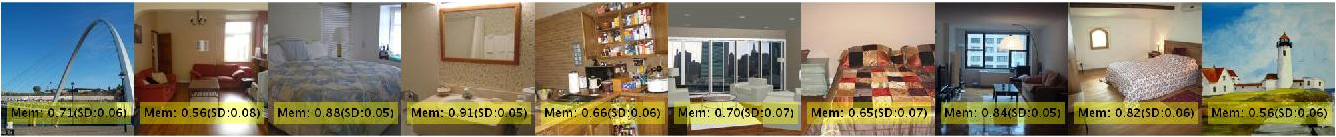}
%    \caption{{\bf Display order 1.}     Images with their memorability scores (Mem) and standard deviation (SD).}
  \end{subfigure}
  \begin{subfigure}[b]{\textwidth}
    \includegraphics[width=\textwidth]{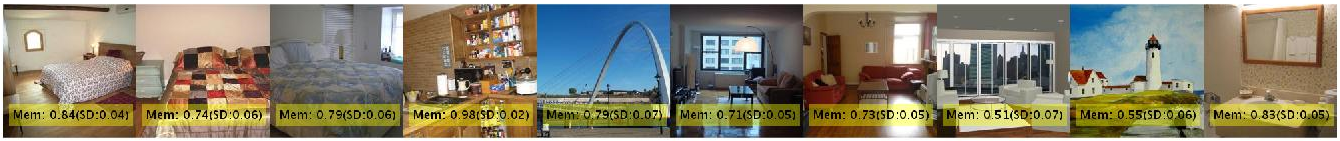}
%    \caption{{\bf Display order 2.}     Images with their memorability scores (Mem) and standard deviation (SD).}
  \end{subfigure}
\centering\caption{{\bf Display order affects image memorability.} 
This figure shows the target images from two different orders of the same set of images (target and fillers), along with their memorability scores (Mem) and the standard deviation (SD).
Depending on the context, the memorability score can dramatically change, e.g., the kitchen.
Conversely, the lighthouse, which is unique in both sequences, gets the same memorability score.
}
\label{fig:displayOrder}
\end{figure*}

%%%%%%%%%%%%%%%%%%%%%%%%%%%%%%%%%%%%%%%%%%%%%%%%%%%%%
%%%%%%%%%%%%%%%%%%%%%%%%%%%%%%%%%%%%%%%%%%%
\vspace{-0.2in}
\subsubsection{Is the image display order important?}
\label{subsec:order}

%1. Describe the practice
Image memorability is commonly measured across random sequences of images, as described before, in order to isolate extrinsic 
effects of image memorability.
Is that the right practice?
Should an image be assigned a single memorability score?
In real life, images are always displayed in some context; for example, when looking at the newspaper, or walking in a museum, the images intentionally appear in a certain order.
In the street, the order of images is not intentional, but it definitely  influences the scenes and objects we will remember or forget.

%2. Challenge #1
To assess the effect of image order on memorability we designed a new version of the ``Memory Game'', in which the only difference is that rather than randomly creating image sequences, we used fixed sets of sequences.
For a fixed set of target and filler images (120 altogether, randomly chosen from Figrim), we created 5 orders.
On average, each target image in each sequence, was scored by 55 participants.
We measured the correlation between groups of 25 participants.
When shown sets of different order, the correlation was low $\rho=0.4$,$\sigma=0.2$, 
while the correlation, when shown the same order, was high $\rho=0.7$,$\sigma=0.1$.
An example why this happens in displayed in Figure~\ref{fig:displayOrder}.
Take for example, the kitchen scene. 
When presented after different scenes (top), its memorability score is $0.66$, however, when presented after a sequence of bedrooms (bottom), its memorability score jumped to $0.98$.

% %3. Our experiment results
% To understand why this is the case, see Figure~\ref{fig:displayOrder}, which shows one example, in which the memorability scores within each sequence are consistent ($0.67$ \& $0.58$), but the consistency between these two sequences is very low ($0.1$).
% The Figure shows the target images in the order presented to the participants, skipping the fillers.
% Take for example, the kitchen scene. 
% When presented after different scenes (top), its memorability score is $0.66$, however, when presented after a sequence of bedrooms (bottom), its memorability score jumped to $0.98$.

% We note that in~\cite{bylinskii2015intrinsic} another extrinsic effect was studied---image context, where context is defined as the images the dataset contains.
% Our study adds a new facet of context---not only the dataset as a whole, but also the order in which the images are presented, affect memorability and should be considered.

This raises the question of how memorability should be measured.
It may well be the case that the current practice of random orders is the right way to somehow alleviates the influence of this extrinsic effect.
% seq 4- 0.67
% seq 5-0.58
% seq 4-5 - 0.1
